# Supplementary material for: ESID: Exploring the Design and Development of a Visual Analytics Tool for Epidemiological Emergencies
Source: arXiv:2304.04635 source file (2023-08-29)
Supplement: Supplementary file 1 [file supplementary_material.pdf]

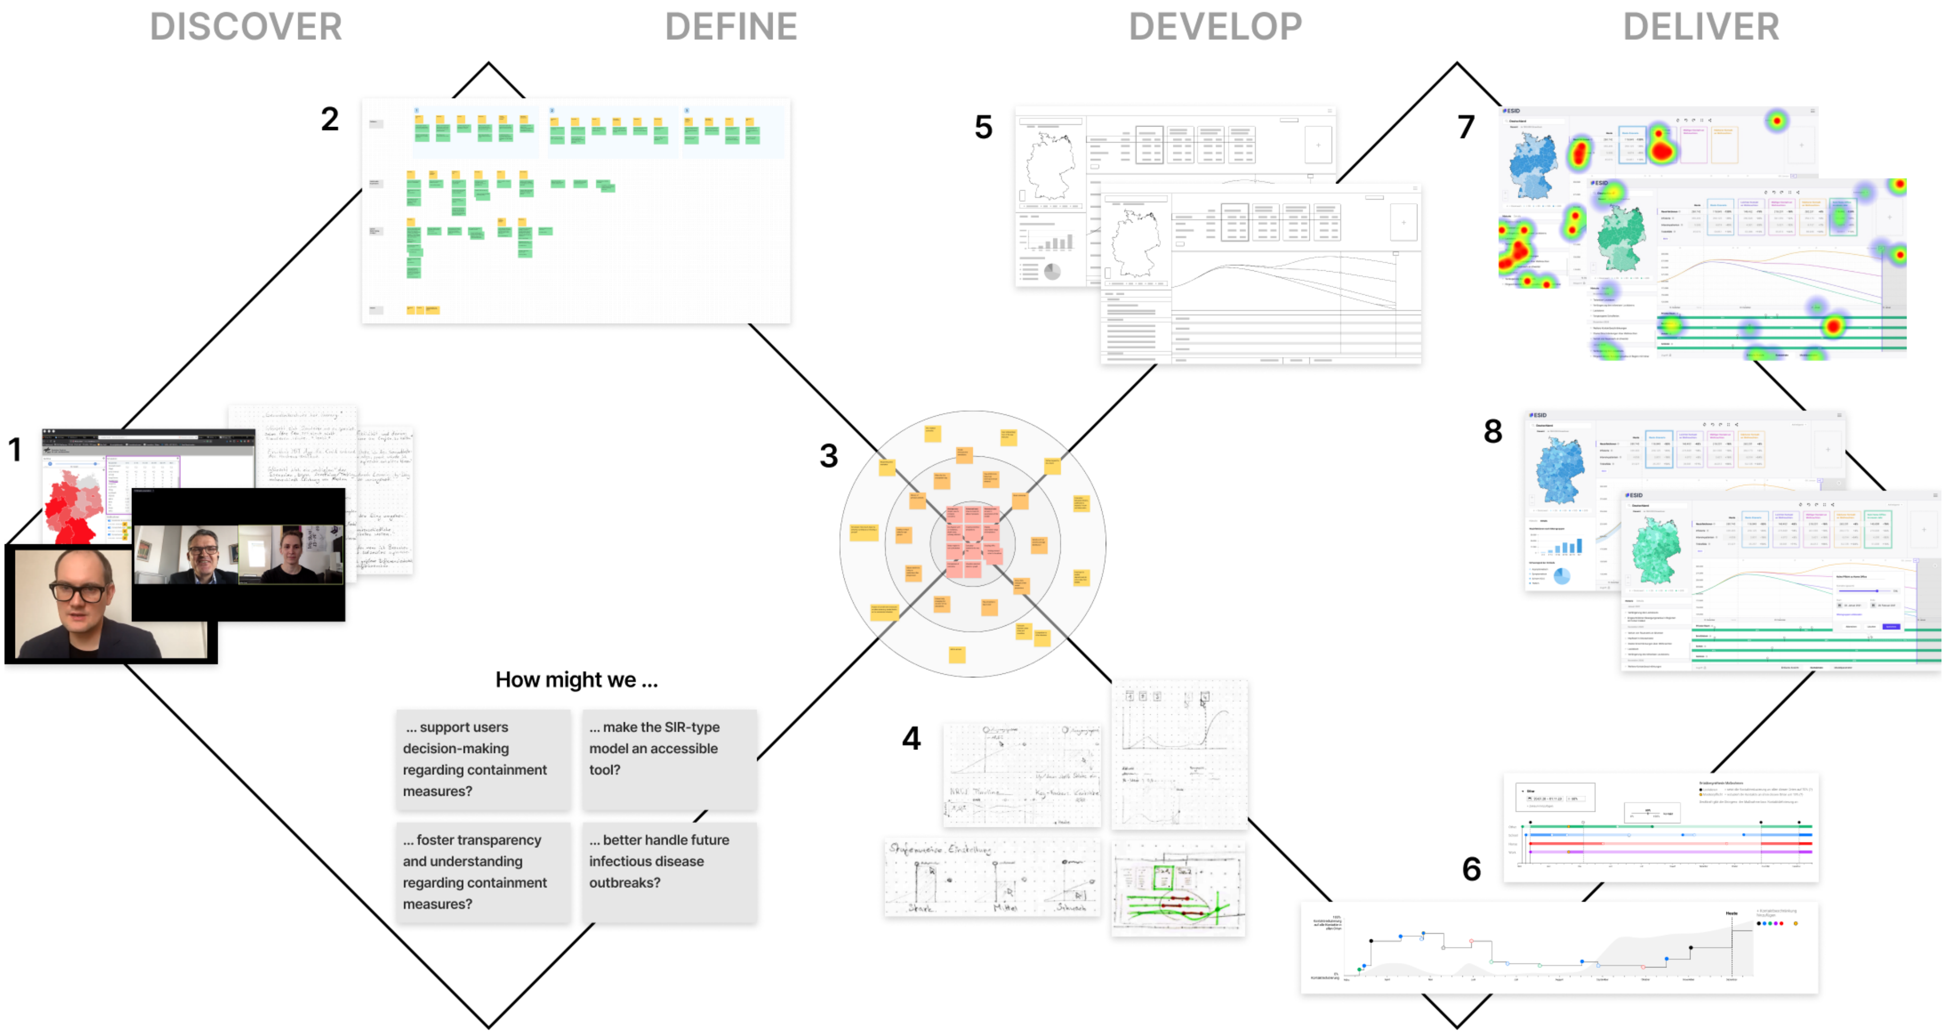
DISCOVER
DEFINE
DEVELOP
DELIVER
1
2
3
4
5
6
7
8
How might we ...
... support users decision-making regarding containment measures?
... make the SIR-type model an accessible tool?
... foster transparency and understanding regarding containment measures?
... better handle future infectious disease outbreaks?

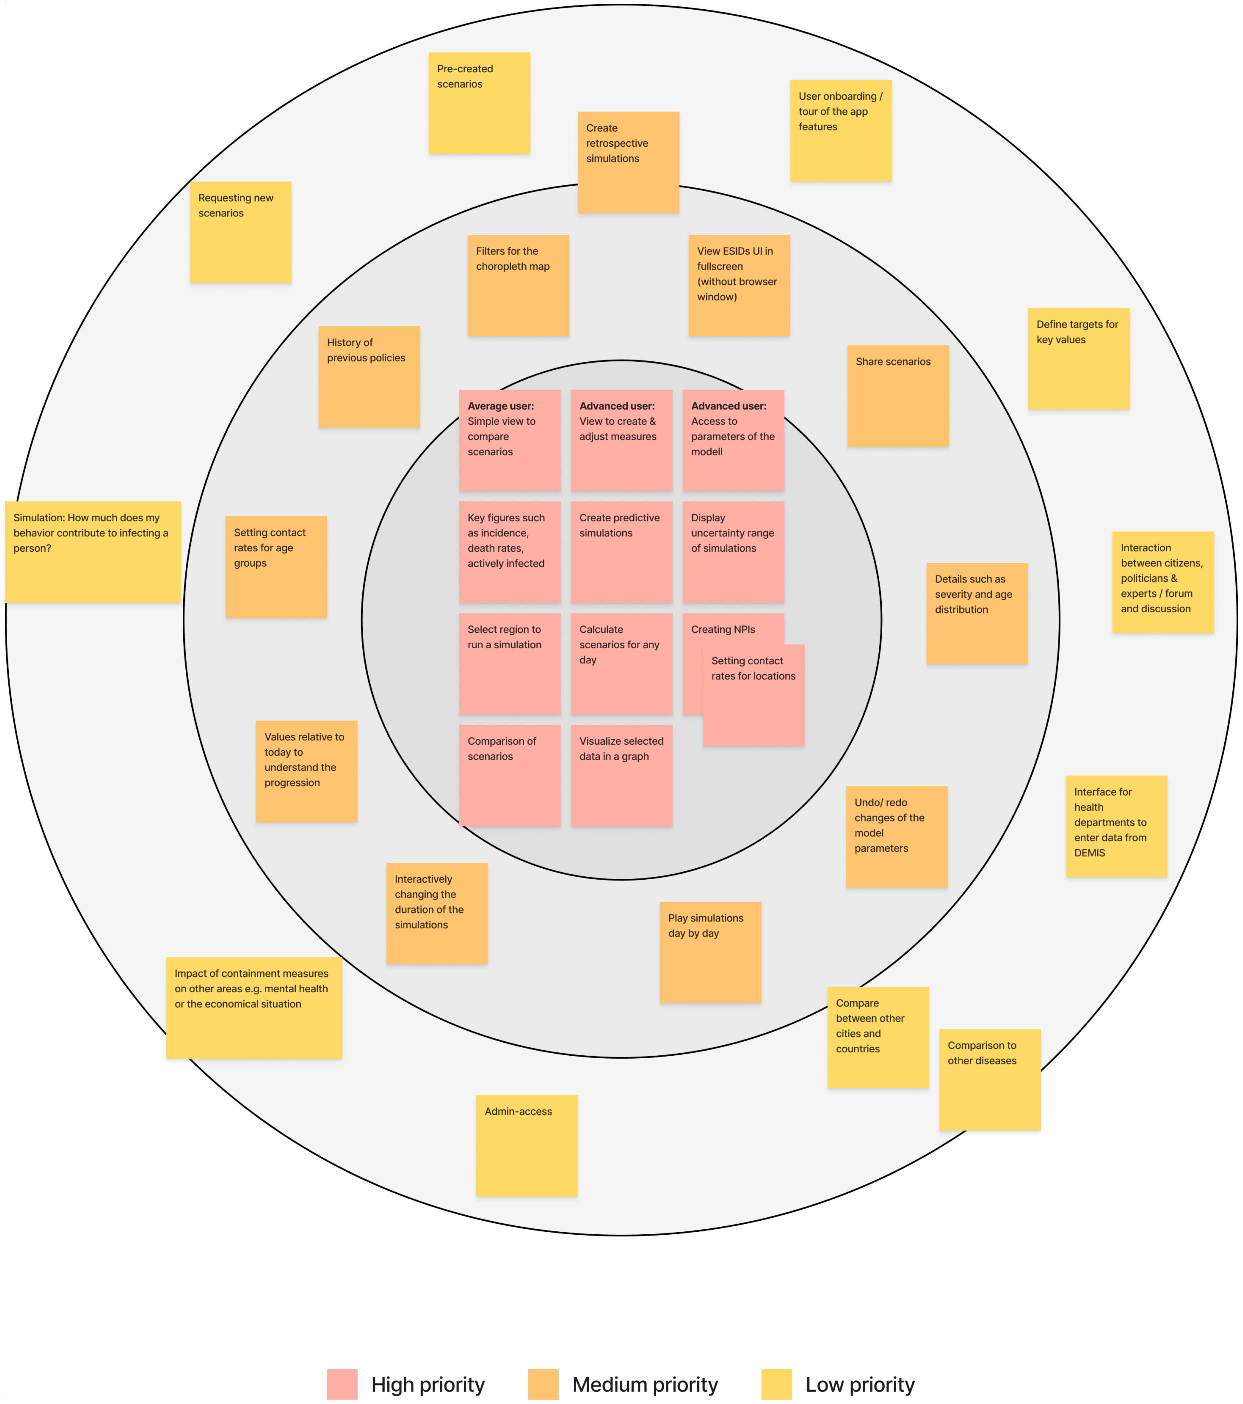

Average user: Simple view to compare scenarios
Advanced user: View to create & adjust measures
Advanced user: Access to parameters of the modell
Key figures such as incidence, death rates, actively infected
Create predictive simulations
Display uncertainty range of simulations
Select region to run a simulation
Calculate scenarios for any day
Creating NPIs
Setting contact rates for locations
Comparison of scenarios
Visualize selected data in a graph
Create retrospective simulations
Filters for the choropleth map
View ESIDs UI in fullscreen (without browser window)
History of previous policies
Share scenarios
Setting contact rates for age groups
Details such as severity and age distribution
Values relative to today to understand the progression
Undo/ redo changes of the model parameters
Interactively changing the duration of the simulations
Play simulations day by day
Pre-created scenarios
User onboarding / tour of the app features
Requesting new scenarios
Define targets for key values
Simulation: How much does my behavior contribute to infecting a person?
Interaction between citizens, politicians & experts / forum and discussion
Interface for health departments to enter data from DEMIS
Impact of containment measures on other areas e.g. mental health or the economical situation
Compare between other cities and countries
Comparison to other diseases
Admin-access
High priority
Medium priority
Low priority

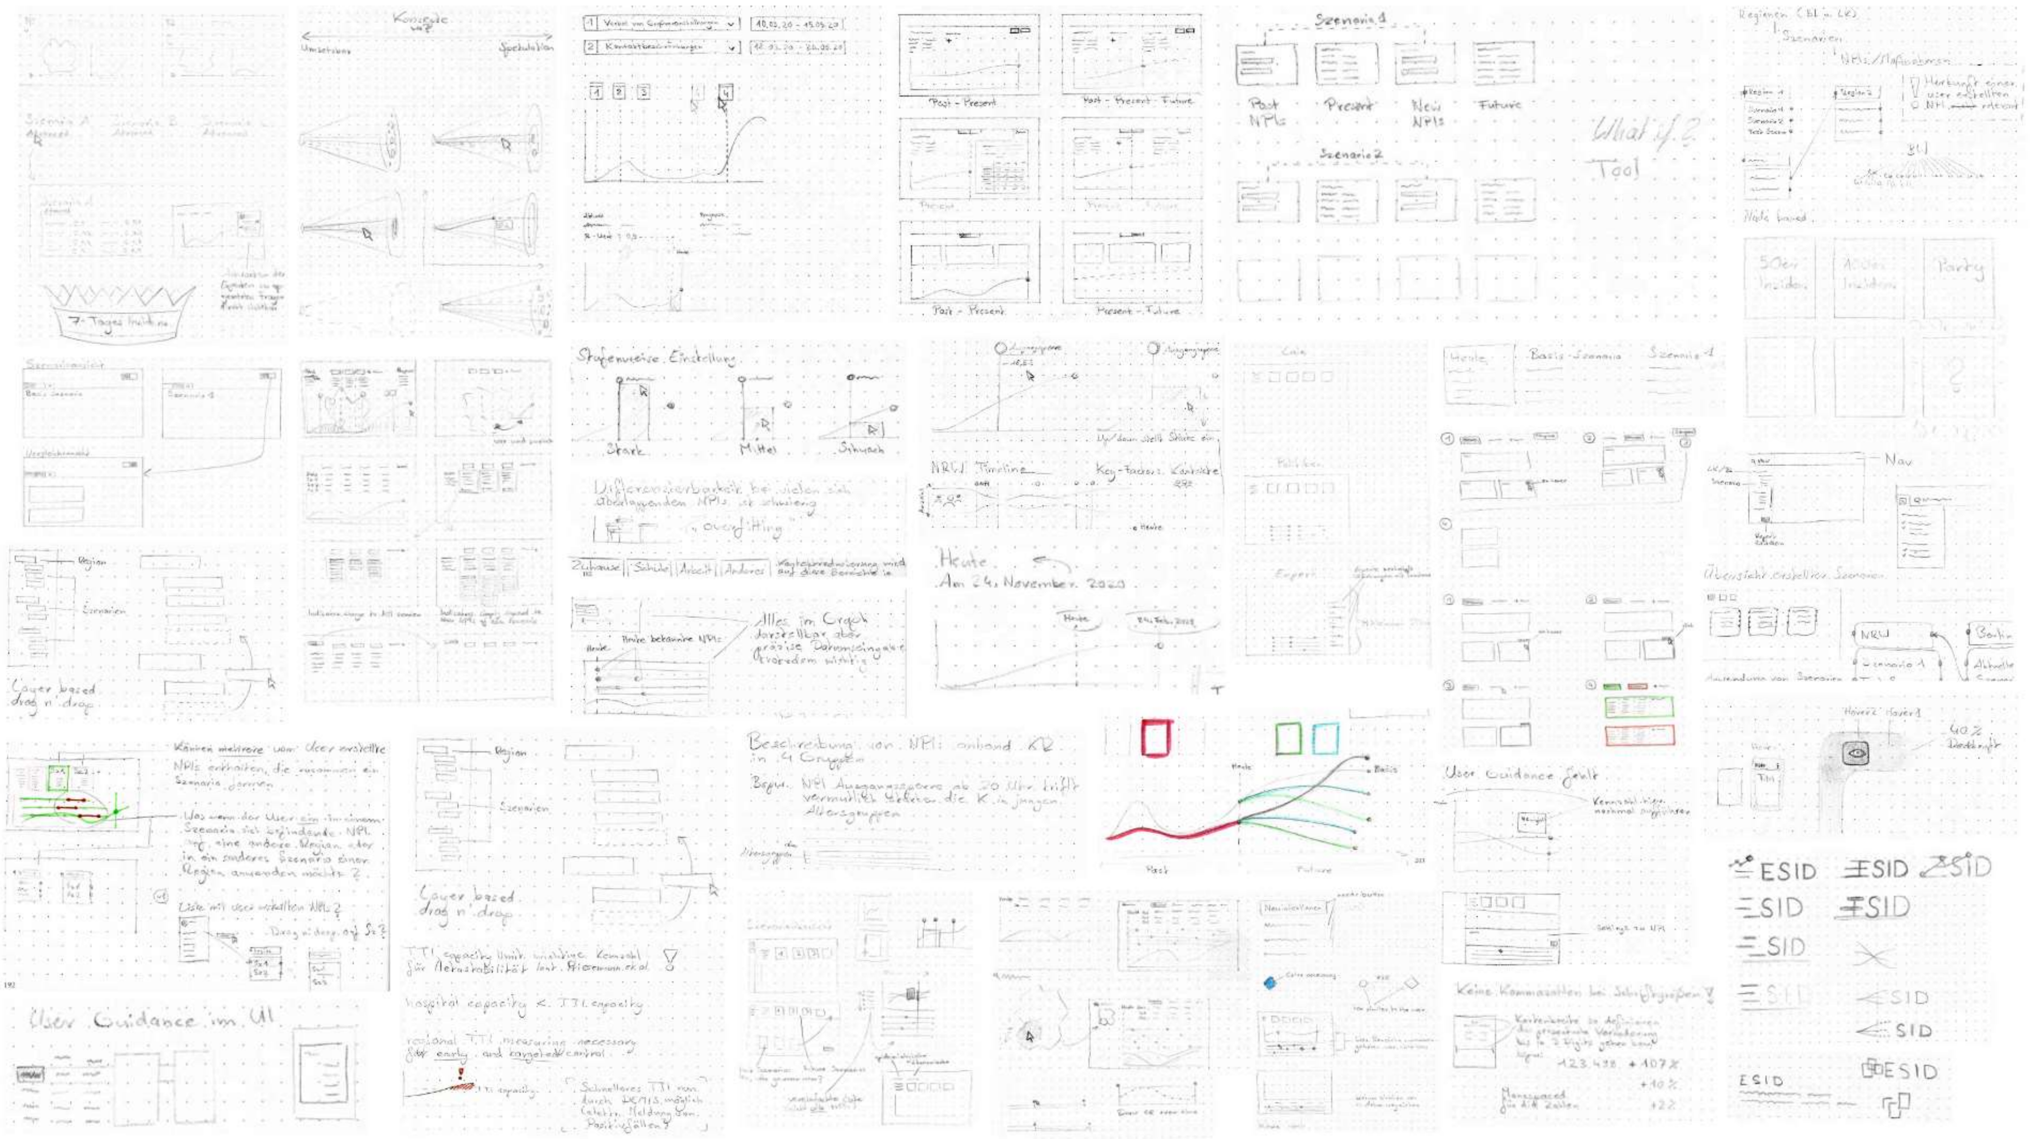
Konzepte
Umsetzbar
Spekulativ
7-Tages Inzidenz
Past - Present
Past - Present - Future
Present - Future
Szenario 1
Szenario 2
Past NPIs
Present
New NPIs
Future
What if?
Tool
Stufenweise Einstellung
Stark
Mittel
Schwach
Differenzierbarkeit bei vielen sich überlagernden NPIs ist schwierig
„overfitting"
Zuhause
Schule
Arbeit
Andere
Alles im Graph darstellbar aber präzise Datumseingabe trotzdem wichtig
NRW Timeline
Heute
Am 24. November 2020
Layer based drag n' drop
Region
Szenarien
Beschreibung von NPIs anhand KR
Past
Future
Basis
User Guidance fehlt
Überblick erstellter Szenarien
Nav
40% Deckkraft
User Guidance im UI
Keine Kommastellen bei Schriftgrößen?
Monospaced für die Zahlen
123.438
+107%
+10%
+22
ESID

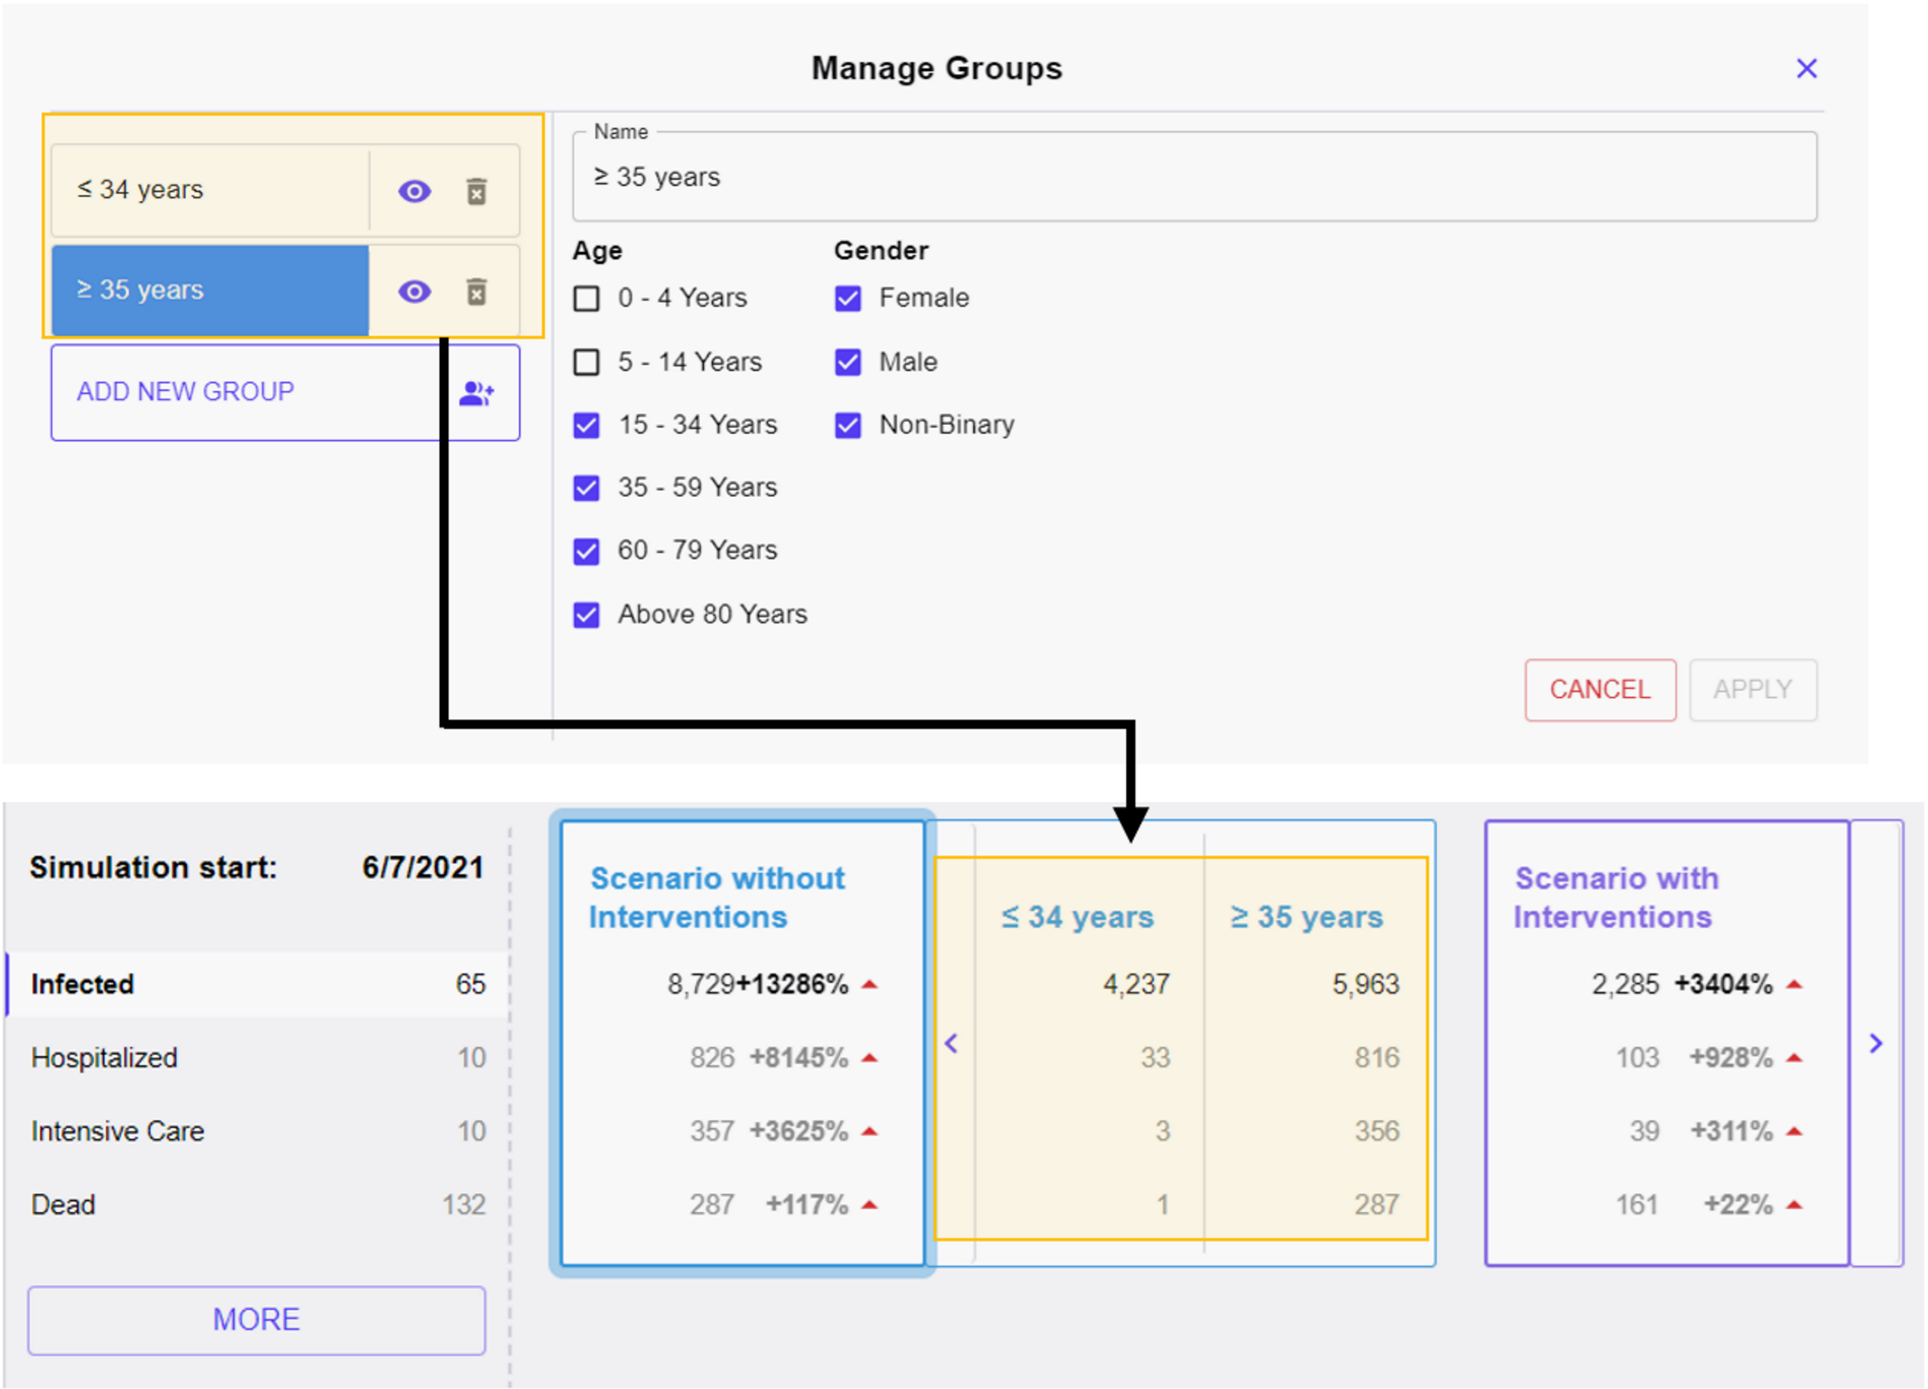
Manage Groups
≤ 34 years
≥ 35 years
ADD NEW GROUP
Name
≥ 35 years
Age
0 - 4 Years
5 - 14 Years
15 - 34 Years
35 - 59 Years
60 - 79 Years
Above 80 Years
Gender
Female
Male
Non-Binary
CANCEL
APPLY
Simulation start: 6/7/2021
Infected 65
Hospitalized 10
Intensive Care 10
Dead 132
MORE
Scenario without Interventions
8,729 +13286%
826 +8145%
357 +3625%
287 +117%
≤ 34 years
4,237
33
3
1
≥ 35 years
5,963
816
356
287
Scenario with Interventions
2,285 +3404%
103 +928%
39 +311%
161 +22%

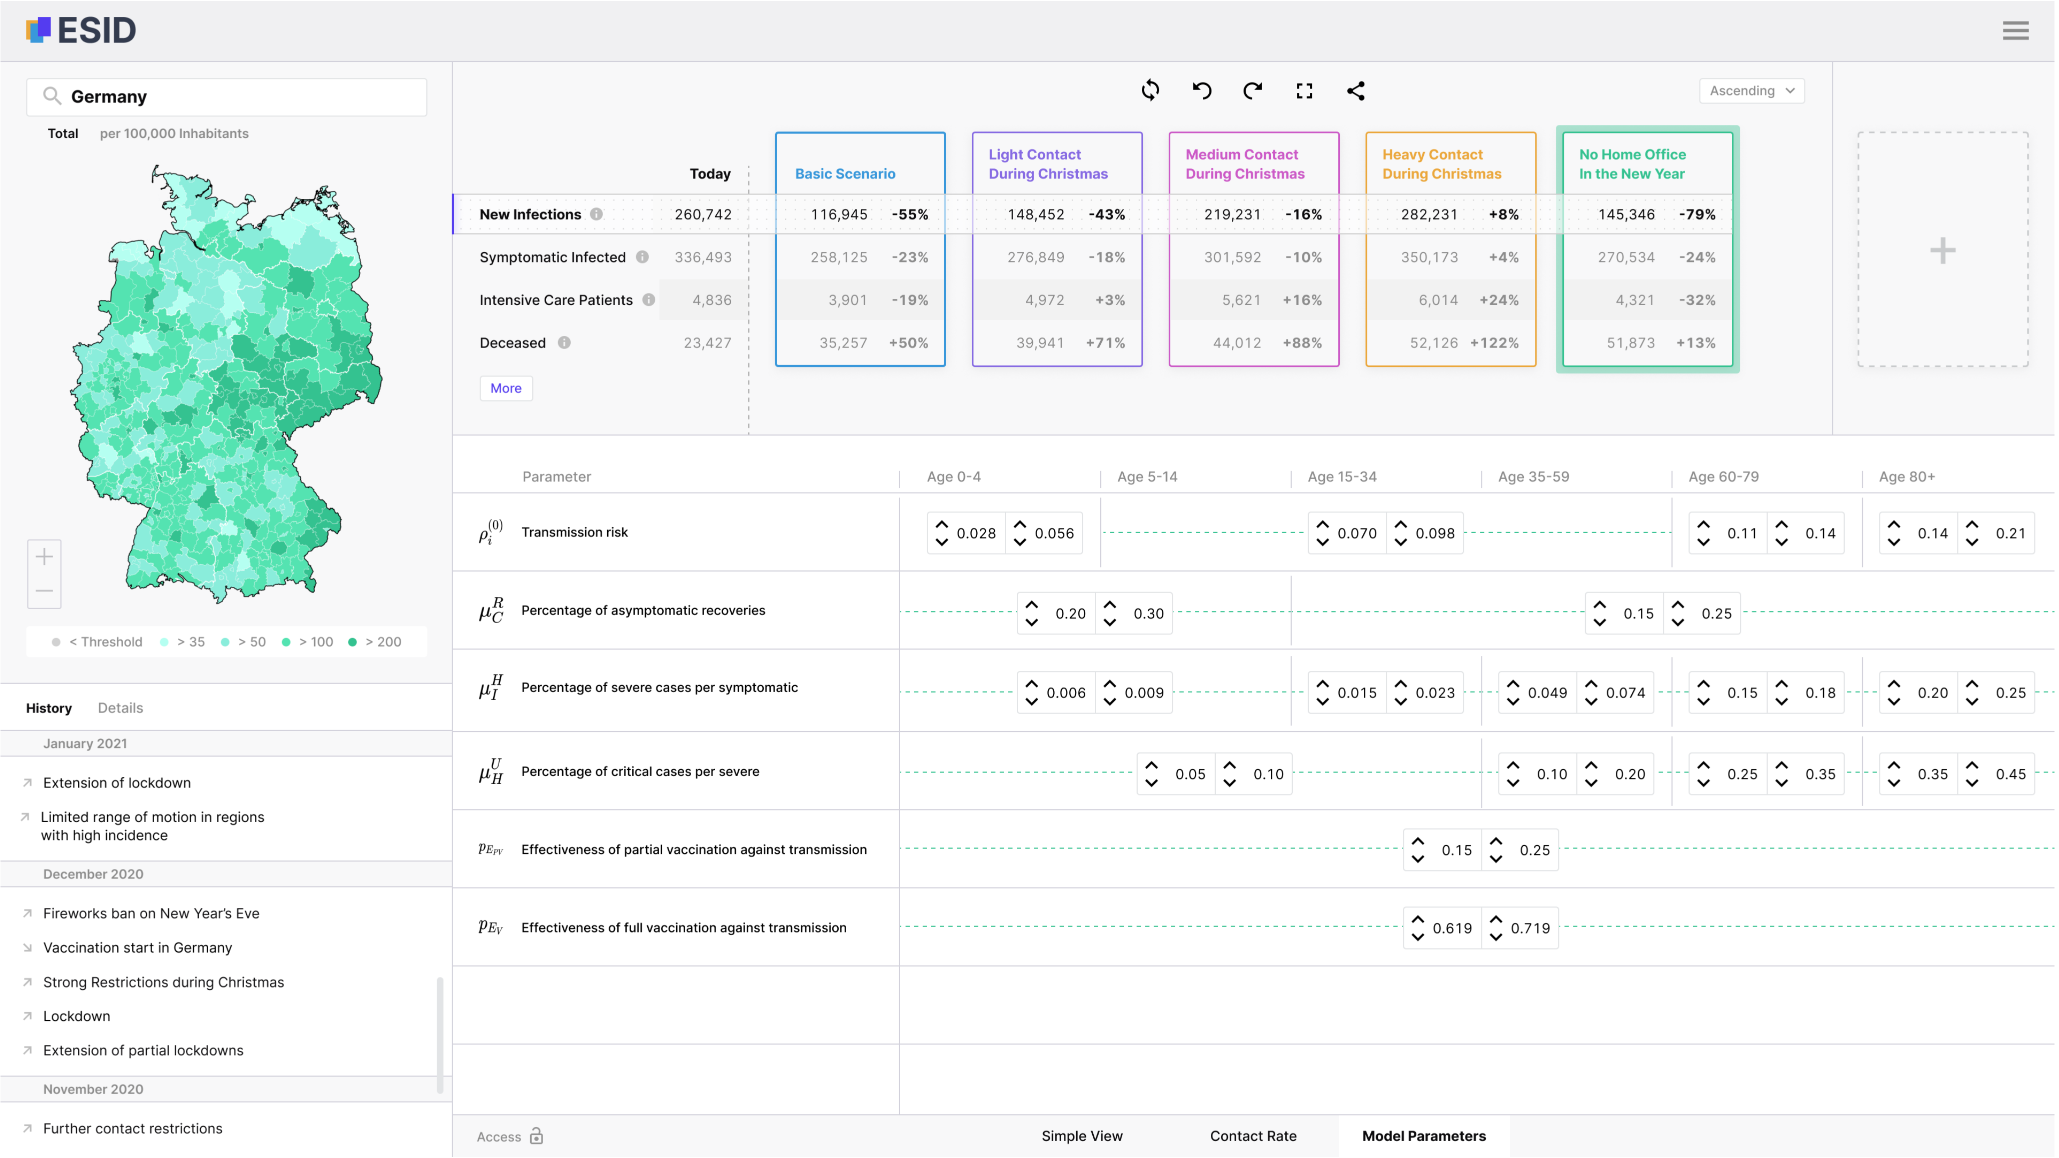
ESID
Germany
Total
per 100,000 Inhabitants
< Threshold
> 35
> 50
> 100
> 200
History
Details
January 2021
Extension of lockdown
Limited range of motion in regions with high incidence
December 2020
Fireworks ban on New Year's Eve
Vaccination start in Germany
Strong Restrictions during Christmas
Lockdown
Extension of partial lockdowns
November 2020
Further contact restrictions
Ascending
Today
Basic Scenario
Light Contact During Christmas
Medium Contact During Christmas
Heavy Contact During Christmas
No Home Office In the New Year
New Infections 260,742 116,945 -55% 148,452 -43% 219,231 -16% 282,231 +8% 145,346 -79%
Symptomatic Infected 336,493 258,125 -23% 276,849 -18% 301,592 -10% 350,173 +4% 270,534 -24%
Intensive Care Patients 4,836 3,901 -19% 4,972 +3% 5,621 +16% 6,014 +24% 4,321 -32%
Deceased 23,427 35,257 +50% 39,941 +71% 44,012 +88% 52,126 +122% 51,873 +13%
More
Parameter
Age 0-4
Age 5-14
Age 15-34
Age 35-59
Age 60-79
Age 80+
$\rho_i^{(0)}$ Transmission risk 0.028 0.056 0.070 0.098 0.11 0.14 0.14 0.21
$\mu_C^R$ Percentage of asymptomatic recoveries 0.20 0.30 0.15 0.25
$\mu_I^H$ Percentage of severe cases per symptomatic 0.006 0.009 0.015 0.023 0.049 0.074 0.15 0.18 0.20 0.25
$\mu_H^U$ Percentage of critical cases per severe 0.05 0.10 0.10 0.20 0.25 0.35 0.35 0.45
$p_{E_{PV}}$ Effectiveness of partial vaccination against transmission 0.15 0.25
$p_{E_V}$ Effectiveness of full vaccination against transmission 0.619 0.719
Access
Simple View
Contact Rate
Model Parameters
